# Supplementary material for: Bounded Situation Calculus Action Theories
Source: arXiv:1509.02012 source file (2015-09-07)
Supplement: Supplementary file 1 [file 90-appendix.tex]

\section{Proof Details}

\endinput

%%% Local Variables:
%%% mode: latex
%%% TeX-master: "main"
%%% save-place: t
%%% End:
